# Supplementary material for: Constant Chemical Potential-Quantum Mechanical-Molecular Dynamics simulations of the Graphene-electrolyte double layer
Source: arXiv:2212.03990 ancillary file (2022-12-09)
Supplement: Supplementary file 1 [file paper_CmuQMMD_SI.pdf]

# Supplementary Material for "Constant Chemical Potential-Quantum Mechanical-Molecular Dynamics simulations of the Graphene-electrolyte double layer"

Nicodemo Di Pasquale *[1], Aaron R. Finney[2], Joshua Elliott[3,4], Paola Carbone[3], and Matteo Salvalaglio[2]

[1] *Department of Chemical Engineering, Brunel University London, Uxbridge, UB8 3PH, United Kingdom*
[2] *Department of Chemical Engineering, University College London, London, WC1E 7JE, United Kingdom*
[3] *Department of Chemical Engineering, University of Manchester, Manchester, M13 9PL, United Kingdom*
[4] *Diamond Light Source, Harwell Science and Innovation Park, Didcot, Oxfordshire OX11 8UQ, United Kingdom*

December 7, 2022

*Corresponding author: nicodemo.dipasquale@brunel.ac.uk

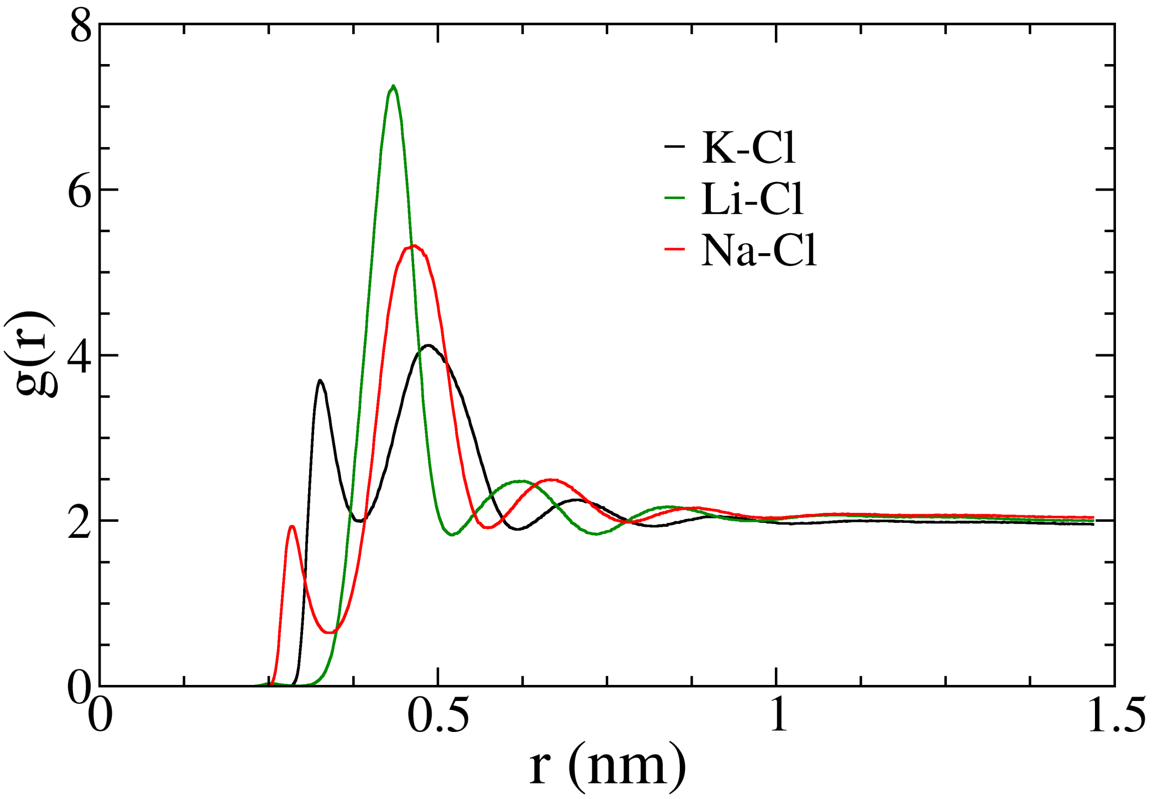


Figure S.1: Radial Distribution Function for the three systems considered

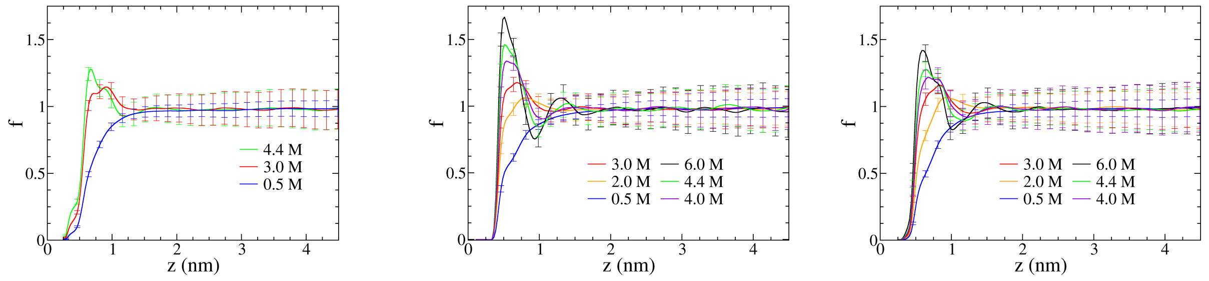


(a) KCl

(b) LiCl

(c) NaCl

Figure S.2: Screening factor as defined in eq. (5) for the three systems and all concentrations considered.

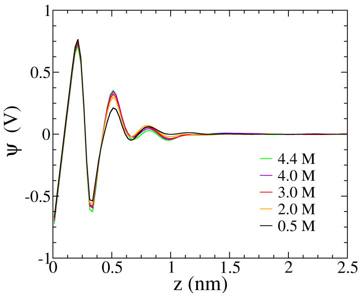


(a) KCl

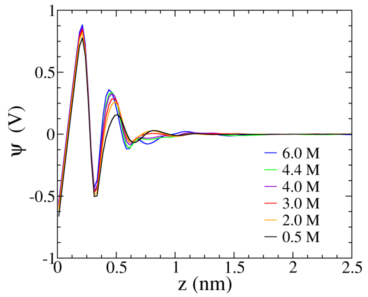


(b) LiCl

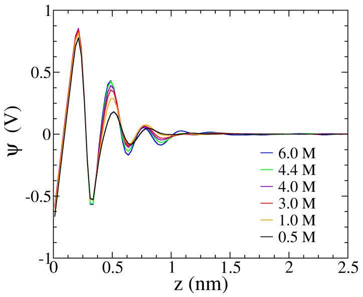


(c) NaCl

Figure S.3: Electrostatic potential as defined in eq. (4) of the main paper for the charged electrode, for the three systems and all the concentrations considered.

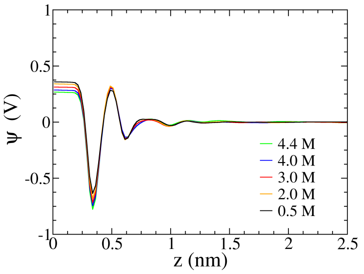


(a) KCl

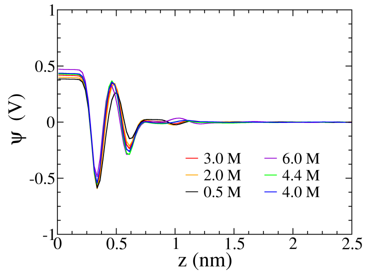


(b) LiCl

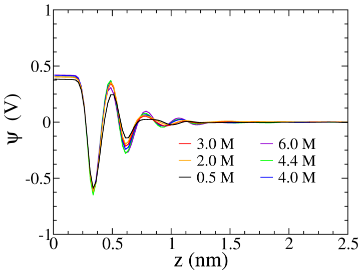


(c) NaCl

Figure S.4: Electrostatic potential as defined in eq. (4) in the main paper for the neutral electrode in all the systems considered.

| | KCl | LiCl | NaCl |
|---|---|---|---|
| concentration | $\Delta\psi^0$ | $\Delta\psi^0$ | $\Delta\psi^0$ |
| 0.5 | 0.359 | 0.385 | 0.383 |
| 2.0 | 0.341 | 0.399 | 0.402 |
| 3.0 | 0.312 | 0.418 | 0.404 |
| 4.0 | 0.286 | 0.436 | 0.416 |
| 4.4 | 0.267 | 0.428 | 0.406 |
| 6.0 | – | 0.471 | 0.420 |

Table S.1: Electrostatic potential drop ($\Delta\psi^0$) across the interface (in V) for the neutral electrode at each ionic system and concentration considered (in M).

|  | KCl | LiCl | NaCl |
|---|---|---|---|
| concentration | $\Delta\psi^-$ | $\Delta\psi^-$ | $\Delta\psi^-$ |
| 0.5 | -0.672 | -0.661 | -0.664 |
| 2.0 | -0.668 | -0.607 | -0.613 |
| 3.0 | -0.688 | -0.584 | -0.593 |
| 4.0 | -0.698 | -0.565 | -0.580 |
| 4.4 | -0.721 | -0.664 | -0.580 |
| 6.0 | – | -0.548 | -0.583 |

Table S.2: Electrostatic potential drop ($\Delta\psi^-$) across the interface (in V) for the charges electrode at each ionic system and concentration considered (in M).

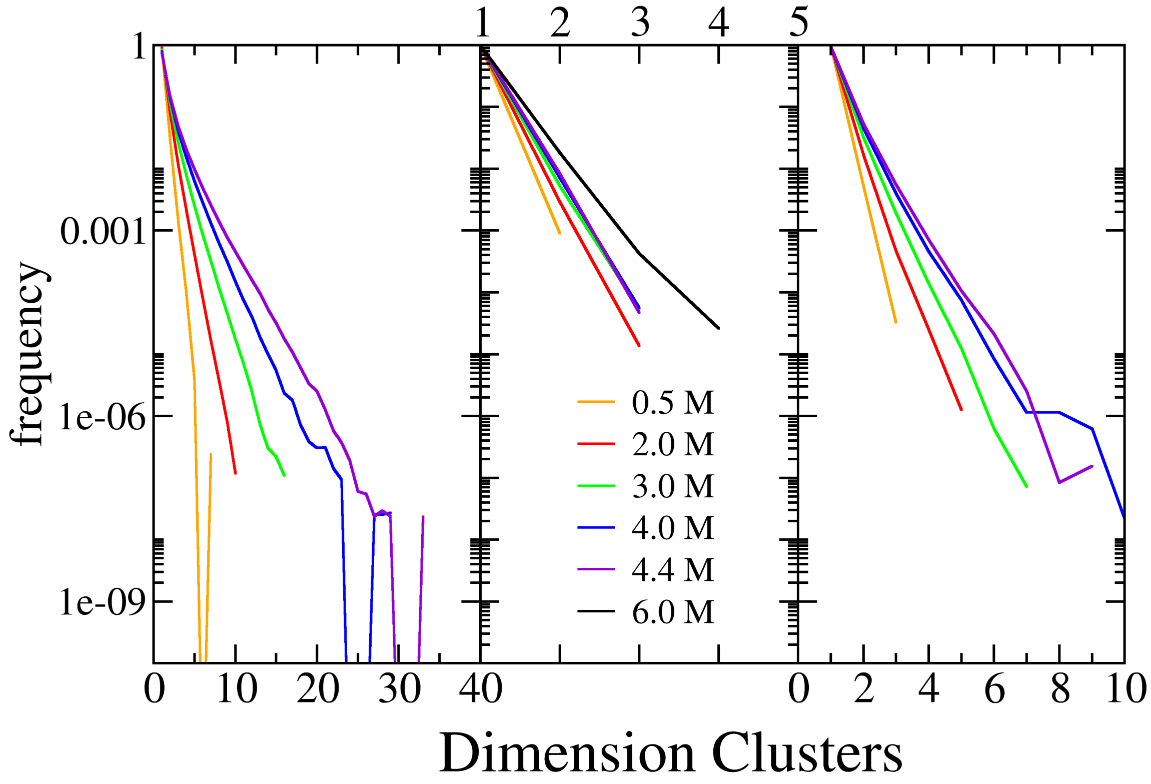


Figure S.5: Histogram of the relative frequency of the cluster of different sizes for all the systems: (from left to right) KCl, LiCl, NaCl and all the concentrations considered.
